# Supplementary material for: MaxUp: A Simple Way to Improve Generalization of Neural Network Training
Source: arXiv:2002.09024 source file (2020-02-20)
Supplement: Supplementary file 1 [file appendix.tex]

\newpage
\appendix
\onecolumn
\section{The proof}
\subsection{Proof of Theorem \ref{thm:weak}}
\label{sec:proof_weak_rademacher}

% \begin{lemma}[Ledoux-Talagrand {\color{red} TODO: citation}]
% $\forall$ function class $\F^\prime$, we have that
% \[
% \Rn[\ell \circ \F^\prime]\le L_{\varphi}\Rn[\F^\prime],
% \]
% \end{lemma}

Define 
\[
\tf_{\th}(\x,y)=\E_{\xxi_{[q]}}\min_{\xxi_{i},i\in[q]}\left[\th^{\top}\left(\x+\xxi_{i}\right)y\right].
\]
Thus when $y=1$, we have 
\begin{align*}
 & \tf_{\th}(\x,y)\\
= & \th^{\top}\x y+\E_{\xxi_{[q]}}\min_{\xxi_{i},i\in[q]}\th^{\top}\xxi_{i}\\
= & \th^{\top}\x y-\E_{\xxi_{[q]}}\max_{\xxi_{i},i\in[q]}\th^{\top}\xxi_{i}.
\end{align*}
Notice that $\th^{\top}\xxi_{i}\sim\mathcal{N}(\boldsymbol{0},\sigma_{\xxi}^{2}\left\Vert \th\right\Vert ^{2})$,
which gives that 
\[
\E_{\xxi_{[q]}}\max_{\xxi_{i},i\in[q]}\th^{\top}\xxi_{i}=G_{q,\left\Vert \th\right\Vert },
\]
where 
\[
G_{q,r}=q\int_{-\infty}^{\infty}s\Phi^{q-1}(\frac{s}{r\sigma_{\xxi}})\phi(\frac{s}{r\sigma_{\xxi}})ds,
\]
and $\Phi(\cdot)$ and $\phi(\cdot)$ is the cumulative/probability
density function of a standard gaussian distribution. Similarly, we
have 
\begin{align*}
\tf_{\th}(\x,y) & =\th^{\top}\x y+\E_{\xxi_{[q]}}\min_{\xxi_{i},i\in[q]}-\th^{\top}\xxi_{i}\\
 & =\th^{\top}\x y-\E_{\xxi_{[q]}}\max_{\xxi_{i},i\in[q]}\th^{\top}\xxi_{i},
\end{align*}
when $y=-1$. Thus we conclude that 
\[
\tf_{\th}(\x,y)=\th^{\top}\x y-G_{q,\left\Vert \th\right\Vert }.
\]
We then bound the Rademacher complexity of function class $\tF$.
\begin{align*}
\Rn[\tF] & =\frac{1}{n}\E_{\h}\left[\sup_{\left\Vert \th\right\Vert \le R}\sum_{i=1}^{n}h_{i}\left(y_{i}\th^{\top}\x_{i}-G_{q,\left\Vert \th\right\Vert }\right)\right]\\
 & \le\frac{1}{n}\E_{\h}\left[\sup_{\left\Vert \th\right\Vert \le R}\sum_{i=1}^{n}h_{i}y_{i}\th^{\top}\x_{i}\right]+\frac{1}{n}\E_{\h}\left[\sup_{\left\Vert \th\right\Vert \le R}\sum_{i=1}^{n}h_{i}G_{q,\left\Vert \th\right\Vert }\right]\\
 & =\Rn[\F]+\frac{1}{n}\E_{\h}\left[\sup_{\left\Vert \th\right\Vert \le R}\sum_{i=1}^{n}h_{i}G_{q,\left\Vert \th\right\Vert }\right]\\
 & =\Rn[\F]+\frac{1}{n}\E_{\h}\left[\sum_{i=1}^{n}h_{i}\mathbb{I}\left\{ \sum_{i=1}^{n}h_{i}>0\right\} G_{q,R}\right]\\
 & =\Rn[\F]+\frac{G_{q,R}}{2n}\E_{\h}\left[\left|\sum_{i=1}^{n}h_{i}\right|\right]\\
 & \le\Rn[\F]+\frac{G_{q,R}}{2\sqrt{n}},
\end{align*}
where the last inequality is by Khintchine's inequality.

% \subsection{Proof of Proposition \ref{prop:half_space}}

% By definition we know $\Delta_{0}(\th)=0$ and $\Delta_{q}(\th)$ is monotonically nondecreasing w.r.t. $q$. We have $\Delta_{q}(\th)\ge0$ for $q\in\mathbb{Z}$.

% Notice that when $\varphi(s)=-s$, we have
% \begin{align*}
%  & \E_{\mathcal{D}}\E_{\xxi_{[q]}}\max_{\xxi_{i},i\in[q]}\ell(f_{\th}(\x+\xxi_{i}),y)\\
% = & \E_{\epsilon \sim \mathcal{N}(0, \sigma^2 I)}\left[-\th^{\top}(\th^{*}y+\epsilon)y\right]-\mathbb{E}_{y\sim\text{Unif}\{-1, +1\}}\E_{\xxi_{[q]}}\min_{\xxi_{i},i\in[q]}\th^{\top}\xxi_{i}y\\
% = & \E_{\mathcal{D}}\ell(f_{\th}(\x),y)+G_{q,\left\Vert \th\right\Vert}.
% \end{align*}

% The second equation holds as no matter $y=\pm 1$, the term $\E_{\xxi_{[q]}}\min_{\xxi_{i},i\in[q]}\th^{\top}\xxi_{i}y$ is always equal to $-G_{q, \|\theta\|}$, with the methods used in Section \ref{sec:proof_weak_rademacher}.

\subsection{Proof of Theorem \ref{thm:cdf}}

Given training set $\{\x_{i},y_{i}\}_{i=1}^{n}$ and choose the $0$-1
loss, $\varphi(s)=\mathbb{I}\{s\le0\}$. We learn $\th$ by minimizing
\[
\frac{1}{n}\sum_{i=1}^{n}\mathbb{E}_{\xxi_{[q]}}\min_{\xxi_{j},j\in[q]}\mathbb{I}\left\{ \th^{\top}(\x_{i}+\xxi_{j})y_{i}\le0\right\} .
\]
Notice that if $y_{i}=1$, we have 
\[
\mathbb{I}\left\{ \th^{\top}\xxi_{j}\le-\th^{\top}\x_{i}\right\} \sim\text{Bernoulli}\left(\Phi\left(\frac{-\th^{\top}\x_{i}}{\left\Vert \th\right\Vert \sigma_{\xxi}}\right)\right).
\]
And thus 
\[
\mathbb{E}_{\xxi_{[q]}}\min_{\xxi_{j},j\in[q]}\mathbb{I}\left\{ \th^{\top}(\x_{i}+\xxi_{j})y_{i}\le0\right\} =1-\left[1-\Phi\left(\frac{-\th^{\top}\x_{i}}{\left\Vert \th\right\Vert \sigma_{\xxi}}\right)\right]^{q}.
\]
If $y_{i}=-1$, we have 
\begin{align*}
\mathbb{I}\left\{ \th^{\top}(\x_{i}+\xxi_{j})y_{i}\le0\right\}  & =\mathbb{I}\left\{ \th^{\top}\xxi_{i}\ge-\th^{\top}\x_{i}\right\} \\
 & =\mathbb{I}\left\{ -\th^{\top}\xxi_{i}\le\th^{\top}\x_{i}\right\} \\
 & \sim\text{Bernoulli}\left(\Phi\left(\frac{\th^{\top}\x_{i}}{\left\Vert \th\right\Vert \sigma_{\xxi}}\right)\right),
\end{align*}
which gives that 
\[
\mathbb{E}_{\xxi_{[q]}}\min_{\xxi_{j},j\in[q]}\mathbb{I}\left\{ \th^{\top}(\x_{i}+\xxi_{j})y_{i}\le0\right\} =1-\left[1-\Phi^{q}\left(\frac{\th^{\top}\x_{i}}{\left\Vert \th\right\Vert \sigma_{\xxi}}\right)\right]^{q}.
\]
And thus we have 
\begin{align*}
 & \frac{1}{n}\sum_{i=1}^{n}\mathbb{E}_{\xxi_{[q]}}\min_{\xxi_{j},j\in[q]}\mathbb{I}\left\{ \th^{\top}(\x_{i}+\xxi_{j})y_{i}\le0\right\} \\
= & 1-\frac{1}{n}\sum_{i=1}^{n}\left[1-\Phi\left(\frac{-\th^{\top}\x_{i}y_{i}}{\left\Vert \th\right\Vert \sigma_{\xxi}}\right)\right]^{q}.
\end{align*}
 
% \section{Can the proposed training method decrease the model class complexity?}
% {\color{red} Unfortunately, for separable data, we cannot improve over max-margin classifier like SVM. So the optimization procedure plays the roles!}

% Generally, we cannot analyze the impact of optimization for all of the objective. Consider some special case?
