# Supplementary material for: MaxUp: A Simple Way to Improve Generalization of Neural Network Training
Source: arXiv:2002.09024 source file (2020-02-20)
Supplement: Supplementary file 2 [file appendix_new.tex]

\subsection{Adversarial Training as Smooth Regularization}

It is worth noticed that, adversarial training can be viewed as a training methods with special data augmentation: the adversarial examples. However, this kind of data augmentation does not aimed at improving the generalization, but for the adversarial robustness. Here, we use the similar idea to show that, when performing adversarial training in $\ell_p$-ball, $p\geq 1$ with small radius $r$, we can view it as introducing an $\ell_q$ regularization of gradient to the original objective, where $\frac{1}{p} + \frac{1}{q} = 1$.

\begin{proposition}[Adversarial Training as Gradient-norm Regularization]
Assume $\ell(f_{\th}(\x), y)$ is second-order differentiable w.r.t $\x$. Define
\begin{align}
    \bar{L}(\x, \vv\theta):=\max_{\|\x^\prime - \x\|_p \leq r} \Lprime.
\end{align}
Then we have that:
\begin{align}
    \bar{L}(\x, \vv\theta) = \L + r\|\nabla_\x \L\|_q + \mathcal{O}(r^2).
\end{align}
\end{proposition}

\begin{proof}
With Taylor expansion, we have that:
\begin{align}
    & \bar{L}(\x, \vv\theta) \nonumber\\
    = & \L + \max_{\|\x^\prime - \x\|_p\leq r}\langle \nabla_{\x} \L, \x^\prime - \x\rangle + \mathcal{O}(\sigma^2)
\end{align}
With Lemma \ref{lem:dual_norm}, we know that the second term is equal to $r\|\nabla_\x \L \|_q$, that finishes the proof.
\end{proof}
\begin{lemma}
\label{lem:dual_norm}
Assume $g$ is a fixed vector in $\mathbb{R}^d$, then 
\begin{align}
    \max_{\|z\|_p\leq 1} \langle g, z\rangle = \|g\|_q.
\end{align}
\end{lemma}
\begin{proof}
This result can be simply derived via the duality of $\ell_p$ norm. We can also use the Lagrangian multiplier, i.e. solve the following optimization problem:
\begin{align}
    \max_{z} \min_{\lambda \geq 0}\langle g, z \rangle - \lambda(\|z\|_p^p - r^p).
\end{align}
Let $g = (g_1, g_2, \cdots, g_d)^\top$ and $z= (z_1, z_2, \cdots, z_d)^\top$. One of the optimal condition for min-max problem is $g - \lambda (z_1^{p-1}, z_2^{p-1}, \cdots, z_d^{p-1}) = 0$. Thus, we can know that when $z = (\frac{1}{\|g\|_q})^{\frac{q-1}{q}}(g_1^{q-1}, g_2^{q-1}, \cdots, g_d^{q-1})^\top$, the original problem $\max_{\|z\|_p\leq 1} \langle g, z\rangle$ get the maximum, which is $\|g\|_q$.
\end{proof}

\subsection{Average Data Augmentation}

\begin{proposition}[AvgUp as Hessian-trace Regularization]
Assume $\mathbb{P}(\cdot|\x) = \mathcal{N}(\x, \sigma^2 I)$ and $\L$ is third-order differentiable w.r.t $\x$. Define
\begin{align}
    \Laug := \E_{\{\x_i'\}_{i=1}^m\sim \P(\cdot|\x)^m} \left [ \frac{1}{m} \sum_{i=1}^m \Lprime \right]. 
\end{align}
\end{proposition}
Then we have 
\begin{align}
    \Laug = \nonumber \L + \sigma^2 \text{trace}(\nabla_{\x \x} \L) + \mathcal{O}(\sigma^3).
\end{align}
\begin{proof}
%still use
This is a simple folklore result. 
By Taylor expansion, 
\begin{align*}
 & \Laug -  \nonumber \L \\
    & ~~~~~ =\mathbb{E}_{\{\x_i^\prime\}_{i=1}^m \sim \mathbb{P}(\cdot|\x)^m}\left[ \frac{1}{m} \sum_{i=1}^m (\Lprime  - \L )\right]\\
    %= &  \L + \mathbb{E}_{\{\x_i^\prime\}_{i=1}^m \sim \mathbb{P}(\cdot|\x)^m}\frac{1}{m} \left[\Lprime - \L \right]\\
     &~~~~~ = \sigma \mathbb{E}_{z\sim \mathcal{N}(0, I)} \left [\langle \nabla_x \L, z\rangle \right] \\
    &~~~~~~~~~~~~~ + \sigma^2 \mathbb{E}_{z\sim\mathcal{N}(0, I)}\left[ z^\top \nabla_{\x \x} \L) z\right]+ \mathcal{O}(\sigma^3)\\
    &~~~~~= \sigma^2 \text{trace}(\nabla_{\x \x} \L) + \mathcal{O}(\sigma^3).
\end{align*}
\end{proof}
This shows that the average loss in \eqref{equ:avgup} tends to penalize the the second order gradient of the loss function, instead of the first order gradient like MaxUp. 
Therefore, AvgUp encourages the loss function $L(\x, \th)$ to behave linearly w.r.t. $\x$, 
and may not be as effective as the smooth regularization of MaxUp in terms of preventing overfitting. 

% As an illustrate, consider the linear regression with loss  $L(\x, \th) = (\x^\top \th - y(x))^2$, where the responsible variable associated with $x$. 
% In this case, the gradient-norm regularization of MaxUp equals equals $\|\nabla_x L(\x,\th)\|_2 = 2\|(\x^\top \th - y(\x))\th \|_2$,
% while the Hessian-trace equals is actually L2 norm of $\theta$.....

% \begin{align}
%     & \nabla_{\x\x} \ell(f_{\th}(\x), y)\\
%     = & \nabla_{\x}(\nabla_{f_{\th}(\x)} \ell(f_{\th}(x), y)\nabla_{\x} f_{\th}(\x))\\
%     = & \nabla_{\x} f_{\th}(\x)^\top \nabla_{f_{\th}(\x)f_{\th}(\x)}\ell(f_{\th}(\x), y) \nabla_\x f_{\th}(\x) + \nabla_{f_{\th}(\x)} (f_{\th}(\x), y) \nabla_{\x \x} f_{\th}(\x)
% \end{align}

% If $\ell(\cdot, \cdot)$ is strongly convex w.r.t the first argument, then the first term is a gradient norm regularization. But the second term depends on local property near $\x$.
